# Supplementary material for: AcTracer: Active Testing of Large Language Model via Multi-Stage Sampling
Source: arXiv:2408.03573 source file (2025-06-11)
Supplement: Supplementary file 1 [file appendix.tex]

\appendix
%\section{Appendix}

\section{Algorithm Details}
\label{appendix:algorithm}

\subsection{1. Vector Representation Extraction}
\label{appendix:vector}

When selecting a target layer as a feature layer for various downstream tasks, studies on classification models typically favor selecting the last hidden layer, assuming it has the most pertinent information regarding their decisions~\cite{li2019boosting, bengio2013better, feinman2017detecting, kim2019guiding, wang2022exploratory}. However, recent research on LLMs indicates that the optimal layer for feature extraction varies depending on the task, with intermediate layers often demonstrating superior performance in various downstream application~\cite{azaria2023the, zou2023representation, gurnee2024language, chen2024inside}. 

%Among related studies, Patchscopes~\cite{ghandeharioun2024patchscope} demonstrates an interesting way to inspect the usefulness of each layer through patching. Given a prompt, it patches one layer of hidden states to another round of inference conditioned on a different prompt and observes the resulting answers. Under their experiments, the intermediate layer still achieves relatively the best performance. This might be because the intermediate layers are responsible for decision-making while the later layer focuses more on token prediction. Motivated by this study, we once wondered whether it is possible to detect a feature layer that is suitable in our cases automatically. As a result, we designed an algorithm shown in Algo~\ref{algo:2}. Generally speaking, we patch a layer given the query prompt and take it into a new inference round conditioned on the empty prompt. We then measure the KL divergence on the output distributions of both cases. Intuitively, the last layer will yield the smallest KL divergence since it preserves all the information for the next-token prediction. However, the layer-KL divergence diagram also presents us with a trade-off similar to the cluster num-inertia diagram, and the elbow point might be an important turning point containing information on the models' high-level decision-making. So, we also conducted experiments based on this strategy.

\input{table/appendix_layer_ablation}

To determine which layer might be more effective, we conducted a preliminary study on Llama-2, comparing the results of feature extraction from the middle layer (16th layer) and the last layer (31st layer). The results are shown in the Table~\ref{tab:appendix_layer_ablation}. The result shows that the middle layer is still the most straightforward layer to choose as the target feature layer. Switching from the middle layer to the last layer resulted in significant performance drops on NQ-open, TruthfulQA-I, and HumanEval, with decreases of 88.29\%, 50.15\%, and 45.12\%, respectively. Nonetheless, we believe it is worth trying more complicated algorithms for automated layer selection in future work. 

%The results for the middle, last, and automated-detected layers (Auto Layer) are shown in the table~\ref{tab:appendix_layer_ablation}.

Another detail in the vector representation extraction phase is the PCA algorithm applied in the feature pre-processing stage. When performing the dimension reduction, we reduced the dimension from 4096 to 64. Our preliminary study shows that 64 is large enough, and a larger value (\eg, 128) can actually slightly hurt the performance. 

%\subsubsection{Automated Search for Cluster Number}
%\label{appendix:cluster_search}

\subsection{2. Automated Search for Cluster Number}
\label{appendix:cluster_search}

\noindent \textbf{Cluster Algorithm} For the cluster search in the second phase of our framework, we leverage Balanced K-means, which is an extended version of naive K-means that formulate the clustering problem as:  

\begin{equation}\label{eq:bal_kmeans}
    \underset{a_1, \ldots, a_{D}}{\max} \sum_{d=1}^{D} -dist(\Vec{h}_{a_d}, \Vec{x}_{d}) \text{ s.t. } \forall k, \sum_{d=1}^{D} \mathbb{1}_{a_d =k} = \frac{D}{K}
\end{equation}

where $a_d \in \{0, \ldots, K\}$ is the cluster assignment index for each data point, $D$ is the number of test points, $dist$ is the distance function, $\Vec{h}_{a_d}$ is the cluster centers, $\Vec{x}_{d}$ is the hidden vector of $d$-th data point, $\mathbb{1}$ is the indicator function. 

Following ~\cite{gururangan2023scaling}, we use Balanced K-means for cluster center estimation and greedy inference when predicting clusters.

\noindent \textbf{Search Algorithm} As we discussed in the main text, finding the appropriate cluster number for analysis is important. We perform a $n$ search to identify the cluster number, and each search includes one Balanced-K-means model fitting. This search is guided by \textit{inertia}, as defined in Eq. \ref{eq:inertia}:

\begin{equation}\label{eq:inertia}
    inertia = \sum_{{d} \in \{{0, \ldots, D}\}} min_{a_d \in \{0, \ldots, K\}} \|\Vec{x}_{d} - \Vec{h}_{a_d}\|^2
\end{equation}

In Eq. \ref{eq:inertia}, $D$ is the number of clusters, $\Vec{x}_{d}$ is the vector representation of each data point, $\Vec{h}_{a_d}$ is the cluster center. 

Our search goal is to identify the elbow point as a cutoff point on the cluster number-inertia curve. Mathematically, given a function $f$, the curvature of $f$ at point $x$ is:

\begin{equation}\label{eq:elbow}
    K_f(x) = \frac{f''(x)}{(1 + f'(x)^2)^{1.5}}
\end{equation}

where $f''(x)$ is the second derivative and $f'(x)$ is the first derivative. The elbow point is the point of maximum negative curvature of the curve. In this work, we utilized Kneedle algorithm~\cite{satopaa2011finding} to find this point. 

To improve the search efficiency of the elbow point, our study further leverages \textit{adaptive} sampling, as proposed by Tinkerer \etal~\cite{nijholt2019adaptive}. This method intensifies sampling frequencies in regions where the inertia function changes rapidly. This is achieved by iteratively dividing a given interval in the direction that can maximize the loss function:

\begin{equation}\label{eq:sample_loss}
    L_{lb, ub} = \sqrt{(ub - lb)^2 + (f(ub) - f(lb))^2}
\end{equation}

where $lb$ and $ub$ are the lower bound and upper bound of the interval, $f(x)$ is the inertia value at the point $x$.

In summary, our cluster number search algorithm is summarized in Algo.~\ref{algo:3}.

\begin{algorithm} \footnotesize
\caption{Search for Target Cluster Number}
\label{algo:3}
\begin{algorithmic}[1]
    \Require LLM \(M\), Test input prompt set \(P\), Target feature layer \(l^{*}\), Search budget \(w\), Search lower bound \(lb\), Search upper bound \(ub\)
    \Ensure Target cluster number at the elbow point
    \State \( SP \leftarrow \text{SPLIT}(lb, ub, w^{i}) \) \Comment{Split search interval into into $w^{i}$ equally spaced points} 
    \State \(ilist \gets \emptyset\) \Comment{Data structure for recording search history}
    
    \For{\(i = 0\) to \(w\)}
        \State \( cn \leftarrow \text{ADP\_SAMPLE}(ilist) \) \Comment{Perform \textit{adaptive} sampling given the past record}
        \State \(S_i \leftarrow \text{CLUSTER}(M, P, l^{*}, cn) \) \Comment{Perform Balanced-Kmeans given the cluster number $cn$ }
        %\State \( ine_{i} = \sum_{i=1}^{k} \sum_{x \in S_{i}} \|x - \mu_i\|^2 \) \Comment{Compute inertia for the cluster}
        \State \( ine_{i} \leftarrow \text{GET\_INERTIA}(S_i)\) \Comment{Compute inertial according to Eq.~\ref{eq:inertia}}
        \State \(ilist \leftarrow ilist \cup (cn, ine_{i}) \)
    \EndFor

    %\State \( elb \leftarrow \text{FIND_ELBOW}(ilist) \)
    \State \(elb \leftarrow \text{FIND\_ELBOW}(ilist) \) \Comment{Perform Elbow-point detection based on search history}
    
    \State \Return \( elb \)
\end{algorithmic}
\end{algorithm}

%\subsubsection{Adaptive Active Sampling Based on Partition}
%\label{appendix:sample}

\subsection{3. Inter-cluster Search}

One additional detail is that in the formal proof part of the MC-UCB algorithm, the authors assume the sample size $N$ satisfies the condition of $N \leq 4K$, where K is the cluster number. As a result, we set the search upper bound based on this condition in Algo~\ref{algo:3}.

\subsection{4. Intra-cluster Search}
\label{appendix:intra}

\input{table/conf_entropy}

Our intra-cluster sampling is guided by the confidence level of LLMs. One important detail is how to aggregate the confidence scores of generated tokens. In this study, we proposed entropy-guided selection criteria for four different kinds of aggregation methods, namely, selecting the first token (first), computing the maximum confidence over the entire generation sequence(\textit{max}), computing the average confidence over the entire sequence(\textit{mean}), computing the geometric mean over the entire sequence (\textit{gmean}). We divide the confidence interval into a histogram consisting of 10 bins and calculate the entropy. The corresponding results for Llama-2 and Code Llama are shown in Table~\ref{tab:llm_entropy_llama2}, and results for Llama-3 are shown in Table~\ref{tab:llm_entropy_llama3}. It is clear that the confidence score distribution varies significantly across different datasets and different models. For example, when evaluating Llama-2 on the HumanEval dataset, the entropy of the max aggregation is zero (i.e., falling into the same bin), while it is 2.733 for the first aggregation. We select the aggregation method according to the maximum entropy across four different methods for each dataset and each model.

%For natural language-based question-answering tasks (\eg, TrivialQA, NQ-open, TruthfulQA), we leverage geometric mean since it better characterizes the probability-driven generation chain of LLMs. For classification tasks (\eg, AGIEval), we directly utilize the first symbol confidence score. For tasks involving math symbols and code blocks (\eg, GSM8K, MBPP, HumanEval), previous studies show that simply aggregating through all tokens might lead to sub-optimal performance for uncertainty estimation~\cite{huang2023look}. As such, we also directly take the confidence of the first non-empty token (\eg, ignoring space). Although it is worth designing a more sophisticated aggregation method,  we think it is beyond the scope of this paper, and we want to avoid over-feature engineering.
\input{table/diptest}

For confidence distribution distance measurement, we use the Wasserstein distance metric and Kolmogorov-Smirnov statistics. As we discussed in the main text, we will perform a dip test to assess the distribution's modality and choose Wasserstein distance for multimodal distribution and Kolmogorov-Smirnov for unimodal distribution. The p-value of the dip test results of Llama-2 and Code Llama are shown in Table~\ref{tab:llm_diptest_llama2} and the the results of Llama-3 are shown in Table~\ref{tab:llm_diptest_llama3}.We set the confidence as 95\%. For a p-value smaller than 5\%, we take it as a multimodal distribution and vice versa. According to all these results, for Llama-2 and Code Llama on AGIEval, TrivialQA, NQ-open, GSM8K, TruthfulQA-I, TruthfulQA-T, HumanEval, and MBPP, we select first + ks, first + wd, gmean + ks, first + ks, gmean + ks, gmean + ks, first + ks	and gmean + ks, respectively. We select first + wd, mean + wd, Mean + ks, max + ks, gmean + wd, gmean + wd, gmean + wd, and first + wd for Llama-3. We additionally conducted ablation studies on the importance of distance metric selections, where we flip the choice of distance measurement in Table~\ref{tab:appendix_diptest_ablation}. It is clear that the appropriate choice of distance measurement is also crucial to the final performance. 

\input{table/ablation_diptest}

\section{Experiment Settings}
\label{appendix:settings}

\textbf{Dataset Description} 

The size of each dataset is shown in Table~\ref{tab:datasize}. We perform our experiments using evaluation framework \textit{Language Model Evaluation Harness}~\cite{eval-harness} for all NLP tasks and implement code generation evaluation with a similar result format to achieve unified I/O for further sampling and analysis.
 
\input{table/dataset_size}

We also report LLMs' performance on evaluated datasets in table~\ref{tab:llm_perf_llama2}, which include experiments of Llama 2-7B on AGIEval, TriviaQA, NQ-open, GSM8K, TruthfulQA-I, TruthfulQA-T, and Code Llama-7B-Python on HumanEval and MBPP. The performance of Llama-3 on all datasets is shown in table~\ref{tab:llm_perf_llama3}. For the evaluation metrics, we use \textit{exact match} for TriviaQA, NQ-open, GSM8K, \textit{accuracy} for AGIEval, probabilities of different fine-tuning models on TruthfulQA, and \textit{pass@1} on MBPP and HumanEval.

\begin{table*}[h] %htbp
    \centering
    
    %\scriptsize
    \resizebox{1.0\columnwidth}{!}{
    \begin{tabular}{cccccccccc}
    \toprule
         Dataset & AGIEval & TrivialQA & NQ-OPEN & GSM8K & TruthfulQA-I & TruthfulQA-T & HumanEval & MBPP  \\ \midrule
         
        %Metric & accuracy & exact match & exact match & exact match & info prob & truth prob & pass@1 & pass@1 \\ \midrule
        
        Mean & 0.2313 & 0.6414 & 0.1889 & 0.1440 & 0.8066 & 0.3390 & 0.3598 & 0.4060 \\ 
        
        Standard deviation & 0.4217 & 0.4796 & 0.3914 & 0.3511 & 0.1523 & 0.3076 & 0.4799 & 0.4911\\ \bottomrule
    \end{tabular}
    }
    \caption{Llama-2 and Code-Llama performance on all evaluated datasets \label{tab:llm_perf_llama2}}
\end{table*}

\begin{table*}[h] %htbp
    \centering
    
    %\scriptsize
    \resizebox{1.0\columnwidth}{!}{
    \begin{tabular}{cccccccccc}
    \toprule
         Dataset & AGIEval & TrivialQA & NQ-OPEN & GSM8K & TruthfulQA-I & TruthfulQA-T & HumanEval & MBPP  \\ \midrule
         
        %Metric & accuracy & exact match & exact match & exact match & info prob & truth prob & pass@1 & pass@1 \\ \midrule
        
        Mean & 0.3022 & 0.7158 & 0.1343 & 0.4792 & 0.7901 & 0.3817 & 0.2561 & 0.3140 \\ 
        
        Standard deviation & 0.4592 & 0.4510 & 0.3410 & 0.4996 & 0.1699 & 0.3263 & 0.4365 & 0.4641\\ \bottomrule
    \end{tabular}
    }
    \caption{Llama-3 performance on all evaluated datasets \label{tab:llm_perf_llama3}}
\end{table*}

%\textbf{Hardware Specification} 

%To conduct our large-scale experiments, we utilize a server
%with AMD 3955WX CPU (3.9GHz), 256GB RAM, and four NVIDIA A4000 GPUs (16GB VRAM of each). The experiments shown in the main text take at least 8,050 CPU Hours and 400 GPU Hours.  

\noindent\textbf{Baseline Description} 

\begin{itemize}[noitemsep, topsep=0pt, parsep=3pt, partopsep=0pt, leftmargin=*]
    \item Confidence-based Stratified Sampling (\csssampling)~\cite{li2019boosting}, which enhances test estimation efficiency by dividing the models' confidence scores across the entire dataset into $k$ sections and then applying stratified sampling according to the confidence distribution within each bin; 
    \item Cross Entropy-based Sampling (\cessampling)~\cite{li2019boosting}, which guides the sampling process through distribution analysis of the last layers' neurons between selected points and the entire test set; 
    \item Practical ACcuracy Estimation (\pacesampling)~\cite{chen2020practical}, which utilizes the MMD-critic algorithm to select the most representative test inputs for test estimation; 
    \item \diffusesampling~\cite{ashury2024label}, a recent approach for label-efficient model selection of LLMs based on clustering analysis of their output text embeddings~\footnote{Model selection and performance estimation share similar settings. By assigning the ground truth label to LLMs' performance, this approach can be effectively adapted for test estimation.};
    \item Rao, Hartley, and Cochran Estimator-based Sampling (\rhcsampling)~\cite{guerriero2024deepsample} guided by Likelihood-based Surprise Adequacy~\cite{kim2019guiding} of internal neurons.

\end{itemize}

\section{Supplementary Experiment Results}
\label{appendix:supplementary}

\subsection{Llama-2 and Code Llama}
We show all the estimation error curves of Llama-2 and Code Llama in Table~\ref{tab:main_result_llama2} from Figure~\ref{fig:llama-2_agieval}
 to Figure~\ref{fig:llama-2_mbpp}.
